# Supplementary material for: Domain Adaptation of Learned Features for Visual Localization
Source: arXiv:2008.09310 source file (2020-08-21)
Supplement: Supplementary file 1 [file supp.pdf]

# Supplementary Material: Domain Adaptation of Learned Features for Visual Localization

Sungyong Baik[†2]
dsybaik@snu.ac.kr
Hyo Jin Kim[1]
kimhyojin@fb.com
Tianwei Shen[1]
tianweishen@fb.com
Eddy Ilg[1]
eddyilg@fb.com
Kyoung Mu Lee[2]
kyoungmu@snu.ac.kr
Chris Sweeney[1]
sweeneychris@fb.com

[1] Facebook Reality Labs
Redmond WA, USA
[2] ASRI, Department of ECE
Seoul National University
Seoul, South Korea

We first visually illustrate our proposed loss terms in the paper (Sec. A). Then, we provide details on the SoftArgMax2D function used in our SoftMatch loss and how it is applied (Sec. B). Next, we present the ablation study on using the visual word constraint in VW-CORAL and CD-SOS losses (Sec. C). Finally, we show more example matching results (Sec. D).

## A Visual Illustration of Introduced Losses

In this section, we detail the three proposed loss terms in the paper, with the help of figures.

### A.1 Visual Vocabulary Construction

As discussed in Sec. 3.4 in the paper, we build the visual vocabulary based on the extracted features from a set of randomly sampled reference images, using the existing feature extraction network (the pre-trained D2-Net [[illegible]] in our case) through K-means clustering (Fig. A).

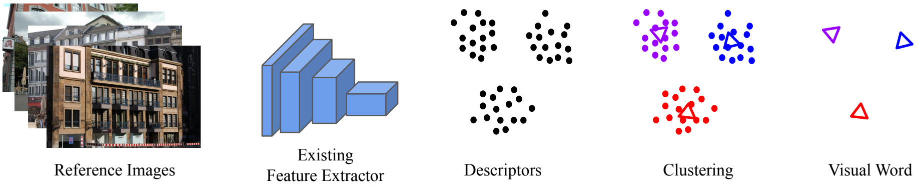


Figure A: Visual vocabulary construction: The existing feature extractor is used to compute the descriptors from the reference images. Then, we perform K-means clustering to obtain visual words.

† Work done while at Facebook Reality Labs.

© 2020. The copyright of this document resides with its authors.
It may be distributed unchanged freely in print or electronic forms.

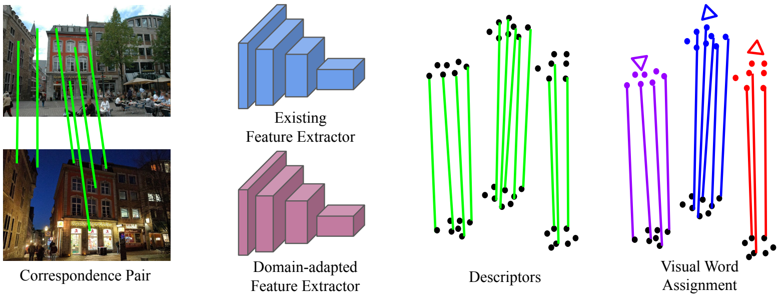


Figure B: Visual word assignment: The source and the target descriptors are extracted from a pair of reference and query images. The source descriptors are assigned to the closest visual words. The visual word assignment for a target descriptor is determined by that of its corresponding source descriptor, based on the training feature correspondences.

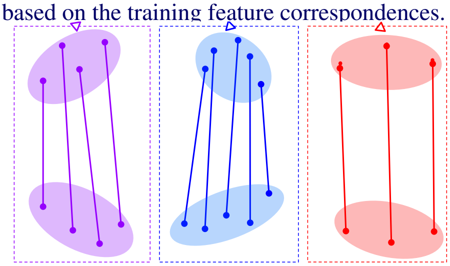

Figure C: Our VW-CORAL loss aligns the distribution of the source descriptors with that of the target descriptors based on the second-order statistics for each visual-word-based group.

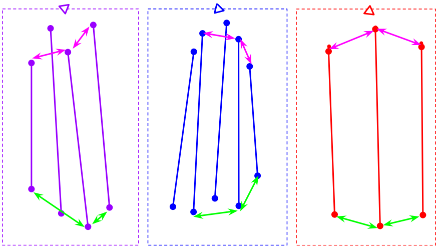

Figure D: Our CD-SOS loss enforces the pairwise distances of target descriptors (green) to be similar to those of the source descriptors (magenta) for each visual-word-based group.

## A.2 Visual Word Assignment

The constructed visual words are then used to group the source descriptors and its corresponding target descriptors that are each extracted from a pair of reference and training image, as in Fig. B. The image pairs are obtained from the registration result of the training images to the reference 3D point cloud. A source descriptor is assigned to the closest visual word. The target descriptor is assigned to the same visual word as its corresponding source descriptor, based on the training feature correspondences (See Sec. 3.3 of the paper).

## A.3 Per Visual Word Correlation Alignment Loss (VW-CORAL)

Fig. C illustrates the VW-CORAL loss that we introduce in Sec. 3.2.2 of the paper. Once the source and the target descriptors are grouped based on their visual word assignment, our VW-CORAL loss minimizes the difference in second-order statistics between the source and the target descriptors for each visual-word-based group separately.

## A.4 Cross-Domain Second Order Similarity Loss (CD-SOS)

Fig. D depicts the concept of our CD-SOS loss detailed in Sec. 3.2.3 of the paper. It enforces the pairwise distances between the target descriptors to be similar to those of the corresponding source descriptors, which are assigned to the same visual words. Compared to the VW-CORAL loss, where the covariance of the distribution is considered, the CD-SOS loss poses more granular supervision by considering the pairwise relationships between the

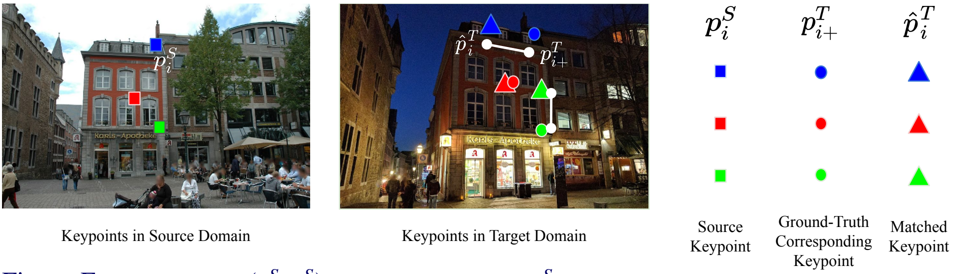


Figure E: For a feature $(\boldsymbol{x}_i^S, \boldsymbol{p}_i^S)$ in the source image $I^S$, our proposed SoftMatch loss penalizes its matched keypoints $\hat{\boldsymbol{p}}_i^T$ in the target image $I^T$ that are far from the actual corresponding keypoints $\boldsymbol{p}_{i+}^T$. The white line represents the distance between the two: $d_i = \|\hat{\boldsymbol{p}}_i^T - \boldsymbol{p}_{i+}^T\|_2$. The larger the distance $d_i$ is, the stronger the loss penalizes the match formed by $\boldsymbol{x}_i^S$.

descriptors in each domain.

## A.5 Soft Matching Loss (SoftMatch)

Fig. E illustrates our SoftMatch loss that is described in Sec. 3.2.4 of the paper. The loss penalizes the matches that disagree with the given pose. For a source descriptor $\boldsymbol{x}_i^S$ at keypoint location $\boldsymbol{p}_i^S$ (squares in Fig. E), we perform a differentiable matching procedure to obtain the estimate of the matched keypoint $\hat{\boldsymbol{p}}_i^T$ (triangles in Fig. E) in the target image. We then compute the distance between $\hat{\boldsymbol{p}}_i^T$ and the actual corresponding point $\boldsymbol{p}_{i+}^T$ (circles in Fig. E) in the image. The actual corresponding point $\boldsymbol{p}_{i+}^T$ is obtained by reprojecting the 3D point $\boldsymbol{c}_i$ that corresponds to the source feature $(\boldsymbol{x}_i^S, \boldsymbol{p}_i^S)$ in the point cloud $\mathcal{C}$ to the target image $I^T$, using the training pose generated as a result of image registration (or the ground-truth pose if available, as in the case of the CSC RobotCar Seasons dataset [2]). Thus, the further away the matched keypoint $\hat{\boldsymbol{p}}_i^T$ is from the actual corresponding target keypoint $\boldsymbol{p}_{i+}^T$, the more it is penalized by the loss.

# B SoftArgMax2D in the SoftMatch Loss

In order to make the whole matching procedure differentiable for the SoftMatch loss (Sec. 3.2.4), we use the SoftArgMax2D function [3] to estimate coordinates of matched keypoints as in Eq. 4 of the main paper. For a given source descriptor $\boldsymbol{x}_i^S$, the coordinates of its matched keypoint $\hat{\boldsymbol{p}}_i^T$ in the target domain image can be obtained by applying the SoftArgMax2D on the 2D match heatmap $\boldsymbol{M}(\boldsymbol{x}_i^S) \in \mathbb{R}^{W \times H}$, where $W$ and $H$ denotes the width and the height of the target image. It is a sparse matrix constructed by matching $i$-th source descriptor $\boldsymbol{x}_i^S$ and all detected local features $(\boldsymbol{x}_j^T, \boldsymbol{p}_j^T)$'s in the target image:

$$\boldsymbol{M}(\boldsymbol{x}_i^S) = [m_{wh}], \tag{1}$$

where each entry $m_{wh}$ is the match score between the source descriptor $\boldsymbol{x}_i^S$ and the target descriptor $\boldsymbol{x}_j^T$ at pixel location $\boldsymbol{p}_j^T = (w,h)$ if the keypoint is detected at that location and 0 otherwise:

$$m_{wh} = \begin{cases} \boldsymbol{x}_j^T \cdot \boldsymbol{x}_i^S & \text{if } (w,h) = \boldsymbol{p}_j^T \\ 0 & \text{otherwise.} \end{cases} \tag{2}$$

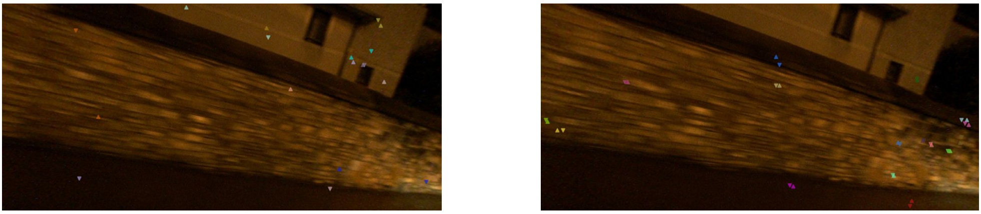

(a) No window (b) Local window

Figure F: The effect of the local window $\boldsymbol{K}$. The figures illustrate the output of SoftArgMax2D when (a) no window is used (uniform weights throughout all locations) and when (b) a local window is applied at the true argmax locations, as in our method. The upward triangles represent the true argmax-regressed coordinates $\hat{\boldsymbol{q}}_i^T$ and the downward triangles the SoftArgMax2D-regressed coordinates $\hat{\boldsymbol{p}}_i^T$.

The SoftArgMax2D function [3] is defined as follows:

$$\hat{p}_{i,x}^T = \sum_{w=1}^{W} \sum_{h=1}^{H} \boldsymbol{K}_{w,h,x} \sigma(m_{wh}), \tag{3}$$

$$\hat{p}_{i,y}^T = \sum_{w=1}^{W} \sum_{h=1}^{H} \boldsymbol{K}_{w,h,y} \sigma(m_{wh}), \tag{4}$$

where $\boldsymbol{K}$ is a weight matrix corresponding to the $xy$-pixel coordinates and $\sigma(m_{wh})$ is the softmax operation on $\boldsymbol{M}(\boldsymbol{x}_i^S)$:

$$\sigma(m_{wh}) = \frac{e^{m_{wh}}}{\sum_{k=1}^{W} \sum_{l=1}^{H} e^{m_{kl}}}. \tag{5}$$

Finally, the coordinates of matched keypoint for the $i$-th source descriptor $\boldsymbol{x}_i^S$ become:

$$\hat{\boldsymbol{p}}_i^T = (\hat{p}_{i,x}^T, \hat{p}_{i,y}^T)^\top. \tag{6}$$

In practice, the weight matrix $\boldsymbol{K}$ is set to be a local window around the true argmax location $\hat{\boldsymbol{q}}_i^T = \text{argmax}_{(w,h)}(\boldsymbol{M}(\boldsymbol{x}_i^S))$ such that it has non-zero values only near $\hat{\boldsymbol{q}}_i^T$. This is because the output of softmax, $\sigma(m_{wh})$ is often multimodal, especially when the 2D match heatmap $\boldsymbol{M}(\boldsymbol{x}_i^S)$ is large. The multimodal input to SoftArgMax2D without the appropriate weight matrix $\boldsymbol{K}$ can result in the regressed coordinates that is far from the true argmax location $\hat{\boldsymbol{q}}_i^T$ (Fig. F (a)). This is undesirable as we want to achieve the similar output to argmax operation for descriptor matching, but in a differentiable manner. Thus, the input to SoftArgMax2D is enforced to be unimodal by setting $\boldsymbol{K}$ to have non-zeros only near the true argmax location $\hat{\boldsymbol{q}}_i^T$ as in the work of Luvizon *et al.* [3], regressing coordinates similar to the argmax location $\hat{\boldsymbol{q}}_i^T$ as a result (Fig. F (b)).

# C Ablation Study on the Visual-Words-Based Constraint

In this section, we assess the effectiveness of applying CORAL and CD-SOS per visual word basis. Table A shows the localization recall using CORAL and CD-SOS loss with and without the visual-word-based grouping, in addition to the correspondence loss $\mathcal{L}_{\text{Corres}}$ on the CSC RobotCar Seasons dataset [2], using an average of 35 training images as in the paper. The results illustrate that applying feature alignment for each visual-word-based group is beneficial, especially for the CD-SOS loss.

Table A: Performance of CORAL and CD-SOS losses with and without the visual word constraint on the CSC RobotCar Seasons dataset [2]

| Losses | VW | Mean Recall |
|---|---|---|
| $\mathcal{L}_{\text{CORAL}}$ [7] | ✗ | 52.0 / 78.8 / 87.9 |
| $\mathcal{L}_{\text{VW-CORAL}}$ | ✓ | **52.4** / 78.9 / 87.8 |
| $\mathcal{L}_{\text{CD-SOS}}$ | ✗ | 52.3 / 78.8 / 87.9 |
| $\mathcal{L}_{\text{CD-SOS}}$ | ✓ | **52.4 / 79.2 / 88.0** |

# D More Qualitative Results

We provide more example matching results for the Aachen dataset [6] and CSC RobotCar Seasons dataset [2] in Fig. G and Fig. H, respectively. In each figure, we show the inlier matches between a pair of retrieved reference image and query image. We compare our method with the pre-trained D2-Net [1] and fine-tuned models. It can be seen that the proposed method improves the matching performance throughout diverse conditions, while the fine-tuned models rarely outperforms the pre-trained model.

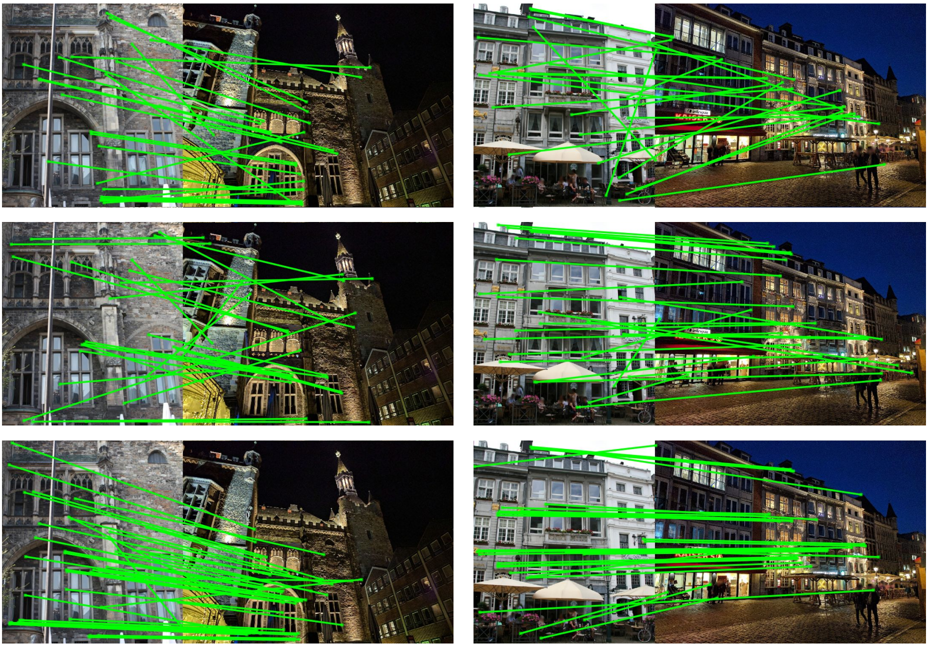

(a) Baseline

(b) Fine-tuned

(c) Ours

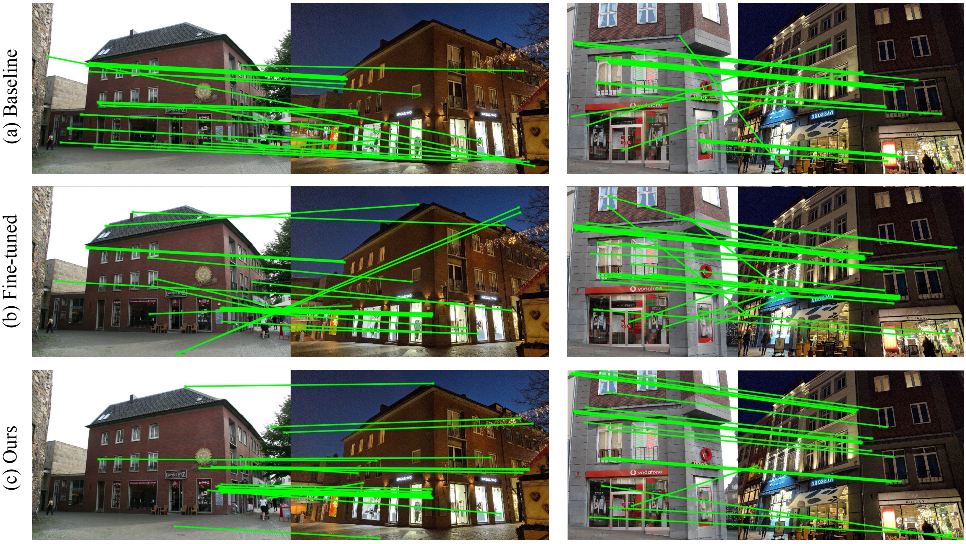


Figure G: Qualitative results on the Aachen Day Night dataset [5] : The inlier matches are visualized for each pair of the retrieved database image (left) and the the query image (right).

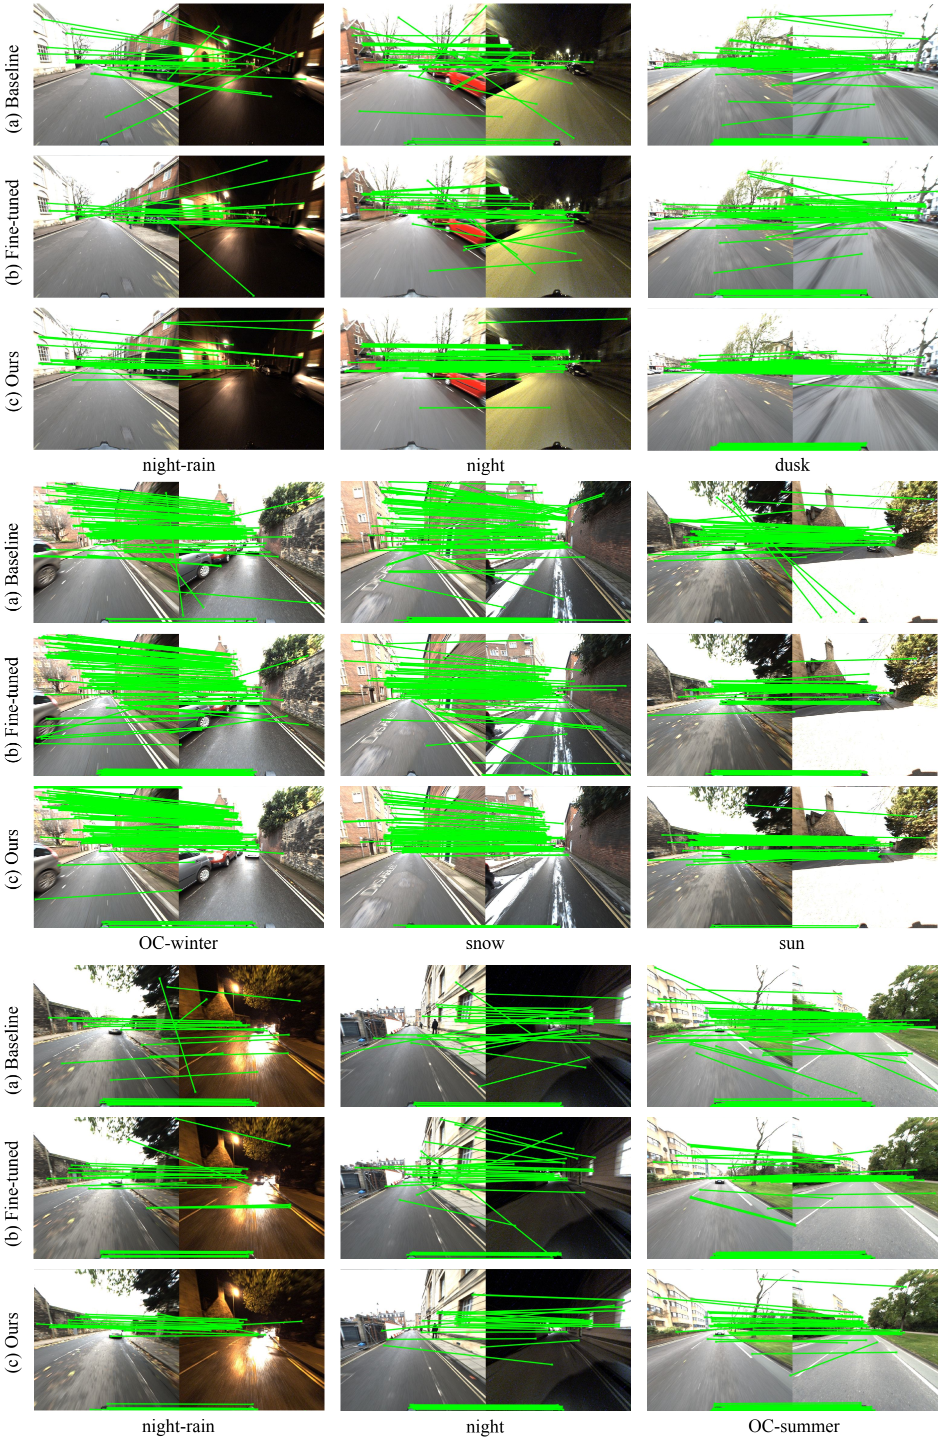


Figure H: Qualitative results on the RobotCar Seasons Dataset [4]: The inlier matches are visualized for each pair of the retrieved database image (left) and the the query image (right).

# References

[1] Mihai Dusmanu, Ignacio Rocco, Tomas Pajdla, Marc Pollefeys, Josef Sivic, Akihiko Torii, and Torsten Sattler. D2-net: A trainable cnn for joint detection and description of local features. In *CVPR*, 2019.

[2] Mans Larsson, Erik Stenborg, Lars Hammarstrand, Marc Pollefeys, Torsten Sattler, and Fredrik Kahl. A cross-season correspondence dataset for robust semantic segmentation. In *CVPR*, 2019.

[3] Diogo C Luvizon, Hedi Tabia, and David Picard. Human pose regression by combining indirect part detection and contextual information. *Computers & Graphics*, 85:15–22, 2019.

[4] Will Maddern, Geoffrey Pascoe, and Paul Newman. 1 year, 1000 km: The oxford robotcar dataset. *International Journal of Robotics Research*, 36(1):3–15, 2017.

[5] Torsten Sattler, Tobias Weyand, Bastian Leibe, and Leif Kobbelt. Image retrieval for image-based localization revisited. In *BMVC*, 2012.

[6] Torsten Sattler, Will Maddern, Carl Toft, Akihiko Torii, Lars Hammarstrand, Erik Stenborg, Daniel Safari, Masatoshi Okutomi, Marc Pollefeys, Josef Sivic, Fredrik Kahl, and Tomas Pajdla. Benchmarking 6dof outdoor visual localization in changing conditions. In *CVPR*, 2018.

[7] Baochen Sun and Kate Saenko. Deep coral: Correlation alignment for deep domain adaptation. In *ECCV*, 2016.
